# Supplementary material for: AnyMoLe: Any Character Motion In-betweening Leveraging Video Diffusion Models
Source: arXiv:2503.08417 source file (2025-03-11)
Supplement: Supplementary file 1 [file X_suppl.tex]

\setcounter{page}{1}
\vspace{5mm}
\maketitlesupplementary

\section*{Overview}
\label{sec:Overview}
In this supplementary material, we present implementation details in Section~\hyperref[sec:A]{A}. Section~\hyperref[sec:B]{B} presents the architecture of scene-specific joint estimator model. Section~\hyperref[sec:C]{C} presents additional results. Visual results and additional comparisons are presented in the supplementary video. Our code will be publicly released upon acceptance.

% For additional results, please visit the project page~\href{https://kwanyun.github.io/lego/}{https://kwanyun.github.io/lego/}.

\section*{A. Implementation Details}
\label{sec:A}

\subsection*{A.1 ICAdapt}
As described in the main paper, to train $D_{adp}$, images are rendered at 30 fps using four different views ($N=4$) of context frames. From these four videos, we sample 16-image clips at 30 fps, 15 fps, and 10 fps using frame intervals of 1, 2, and 3, respectively. This fps information is passed through the fps embedding layer of $D_{adp}$ as a control parameter for video speed. The dataset gathering process is outlined in Algorithm~\ref{alg:ICAdapt_data}. Using these clips, each consisting of 16 images, ICAdapt is conducted for 500 steps with a learning rate of 1e-5, which requires approximately one and a half hours on an Nvidia A6000 GPU. During the ICAdapt process, the video captioning model~\cite{yu2024eliciting} is used once, with the same text prompt applied throughout the entire process, because the animation is played within a single scene.

\subsection*{A.2 Scene-specific joint estimator}
Scene-specific joint estimator $\mathcal{E}_{scene}$ is trained using three views ($N=3$) in addition to the rendered keyframes with the weight $w=3$. As shown in Figure 5 of the main paper, 2D and 3D features are extracted from rendered images. For 2D features, DINOv2~\cite{radford2021learning} is used. Recently,~\citet{darcet2023vision} showed that training DINOv2 with register tokens can reduce high-norm outliers, leading to improved stabilization. Thus we employed them for 2D features. For 3D-aware features, we employed another DINOv2 variant Fit3D~\cite{yue2025improving}, which is also DINOv2 varient, finetuned at 3D scenes. The training was conducted for 3500 steps, which required around 3.5 hours on an Nvidia A6000 GPU. The detailed model architecture of Scene-specific joint estimator will be presented in Section~\hyperref[sec:B]{B}.

\begin{algorithm}[t]
\caption{Gathering video clips from context frames}
\begin{algorithmic}[1]
\Require $N$: Number of views (e.g., $N = 4$)
\Require $N_{fpv}$: Total number of frames per view
\Require $k$: Number of frames per clip (e.g., $k = 16$)
\Require $S$: List of frame intervals for sampling (e.g., $S = [1, 2, 3]$)
\Ensure $Clips$: A list of sampled clips
\State Initialize $Clips \gets []$
\For{$v \gets 1$ to $N$} \Comment{Iterate through all views}
  \ForAll{$s \in S$} \Comment{Iterate through all sampling}
    \For{$start \gets 0$ to $N_{fpv} - k \cdot s$}
      \State $clip \gets [start + i \cdot s \ \textbf{for} \ i \in \{0, 1, ..., k-1\}]$
        \State $Clips \gets Clips \cup \{clip\}$ 
    \EndFor
  \EndFor
\EndFor
\State \Return $Clips$
\end{algorithmic}\label{alg:ICAdapt_data}
\end{algorithm}

\subsection*{A.3 Two-stage Inference}
Two-stage inference is conducted to generate video frames that follow the given context and produce smooth motion. This process is written in Algorithm~\ref{alg:two_stage_video_generation}. In the first stage, a coarse video at 5 fps is generated, with each inference covering a three second segment because $D_{adp}$ outputs 16 frames at a time. In the second stage, a fine video at 15 fps is generated, with each inference covering one second segment. The process ensures both contextual alignment and smooth motion. We conducted an experiment to measure inference time. As shown in Table~\ref{tab:time}, two-stage inference has O(N) time complexity for input keyframes.

\vspace{-2mm}
\begin{table}[h]
    \centering
    \caption{Two-stage inference time for 15fps videos.}
    \vspace{-2mm}
    \label{tab:time}
    \scalebox{0.8}{
        \begin{tabular}{ccccccc}
            \hline
            \textbf{Generated frames} &  15 & 30 & 45 & 60 & 75& 90  \\ \hline
            Inference time (Minutes)        & 2.43 &3.58 & 4.78 & 5.97 & 7.13 & 8.08 \\ \hline
        \end{tabular}
    }
\end{table}
\vspace{-2mm}

\begin{algorithm*}
\begin{minipage}{\linewidth}
\centering
\caption{Two-Stage Video Generation with Context Guidance}
\begin{algorithmic}[1]
\Require $D_{adp}$: Fine-tuned video diffusion model  
\Require $I_0, I_N$: First and last keyframes of the target video  
\Require $Total$: Total time in seconds for the video to generate  
\Require $I_m$: Context frames for guidance, where $M_1 \leq m \leq M_2$, $M_2 < N$
\Ensure Final video with interpolated smooth motion
\State \textbf{Stage 1: Coarse Video Generation with Contextual Interpolation}
\For{$t_{vid} \in \{0, 1, \dots, Total-3\}$} \Comment{Iterate over each second (overlap occurs)}
    \State Initialize noisy latent $z_{n_t}$
    \For{$t \gets T$ to $0$} \Comment{Backward diffusion process}
        \State Denoise $z_{n_{t+1}}$ to obtain $z_{n_t}$
        \If{conditioning}
            \State Replace parts of $z_{n_t}$ with $\mathcal{E}_{vae}(I_m) + \epsilon_t$, where $I_m$ are guidance frames
            \State Update $z_{n_t} \gets z'_{n_t}$ \Comment{Refine latents using guided inpainting}
        \EndIf
    \EndFor
    \State Decode $z_{n_0}$ to obtain coarse video $I_n$
    \State Update $I_m$ to include $I_n$ for future iterations
\EndFor
\State Generate a coarse video with sparse frames: $\{I_0, I_1, \dots, I_{N-1}, I_N\}$
\State \textbf{Stage 2: Fine Video Generation with Higher Frame Rate}
\For{$t_{vid} \in \{0, 1, \dots, Total-1\}$ (smaller intervals)} \Comment{Generate finer frames}
    \State Use $D_{adp}$ with keyframes and generated frames from Stage 1 as guidance
    \State Apply the same guided inpainting technique as in Stage 1
    \State Generate intermediate frames between keyframes and coarse frames
\EndFor
\State Combine all frames to produce a high-frame-rate video
\State \Return Final video
\end{algorithmic}\label{alg:two_stage_video_generation}
\end{minipage}
\end{algorithm*}

\subsection*{A.3 Motion video mimicking}
Motion video mimicking is performed to generate motion that follows the generated video. We use joint loss, image loss, and regularization loss, as described in Eq. 3 of the main paper. The entire optimization process is conducted in a single view ($N=1$), over 100 steps per sequence. This process is performed in batches to achieve faster optimization. For an 8-second video with 2 seconds of context frames, the batch size is 6, and the optimization process is repeated 14 times to fill the in-between frames.

\section*{B. Model Architecture}
\label{sec:B}

\begin{figure*}[t]
\centering
\vspace{3mm}
\includegraphics[width=\linewidth]{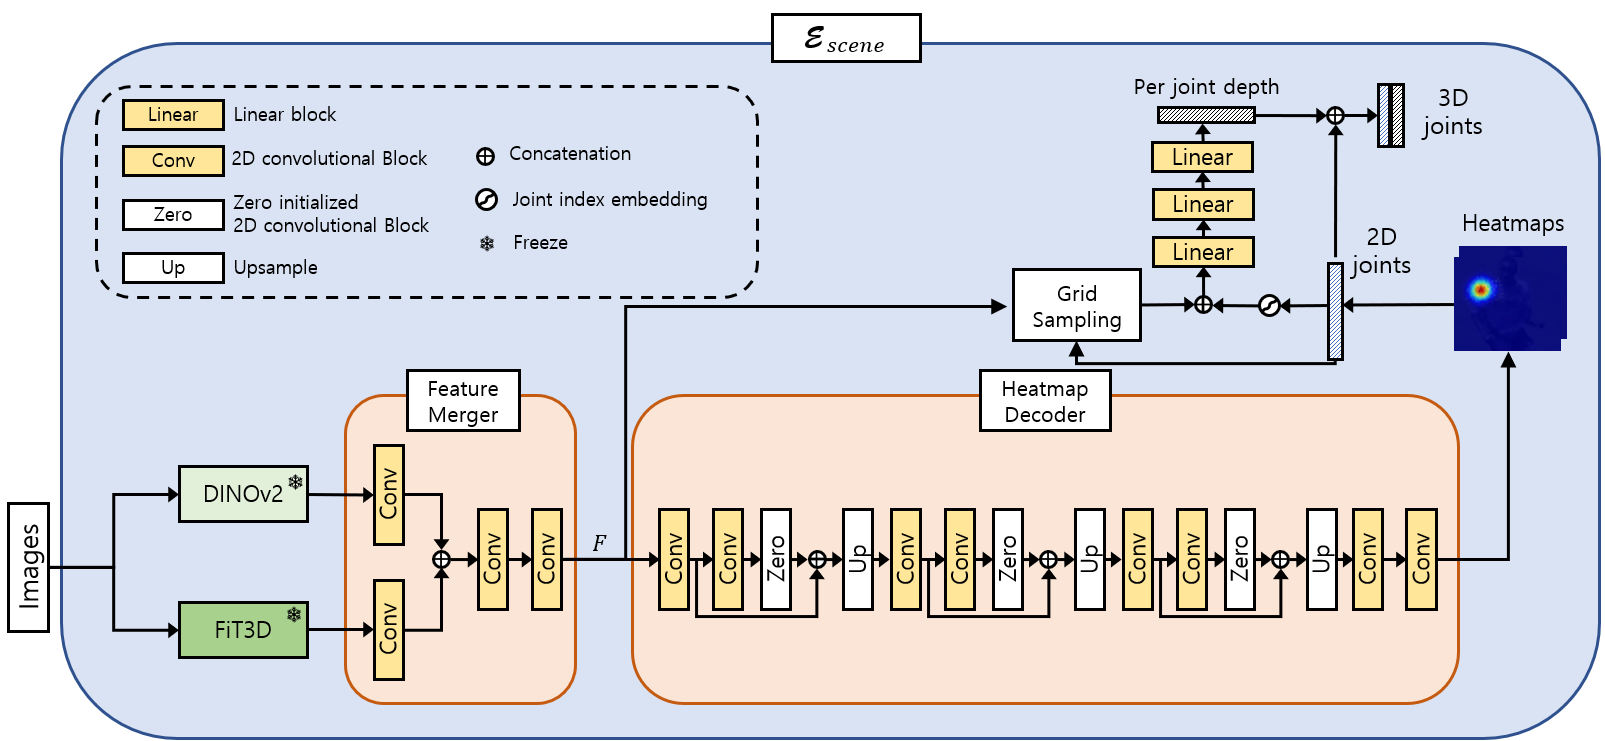}
\caption{Architecture of scene specific joint estimator.}
\label{fig:x_joint}
\end{figure*}

\begin{figure*}[t]
\centering
\includegraphics[width=\linewidth]{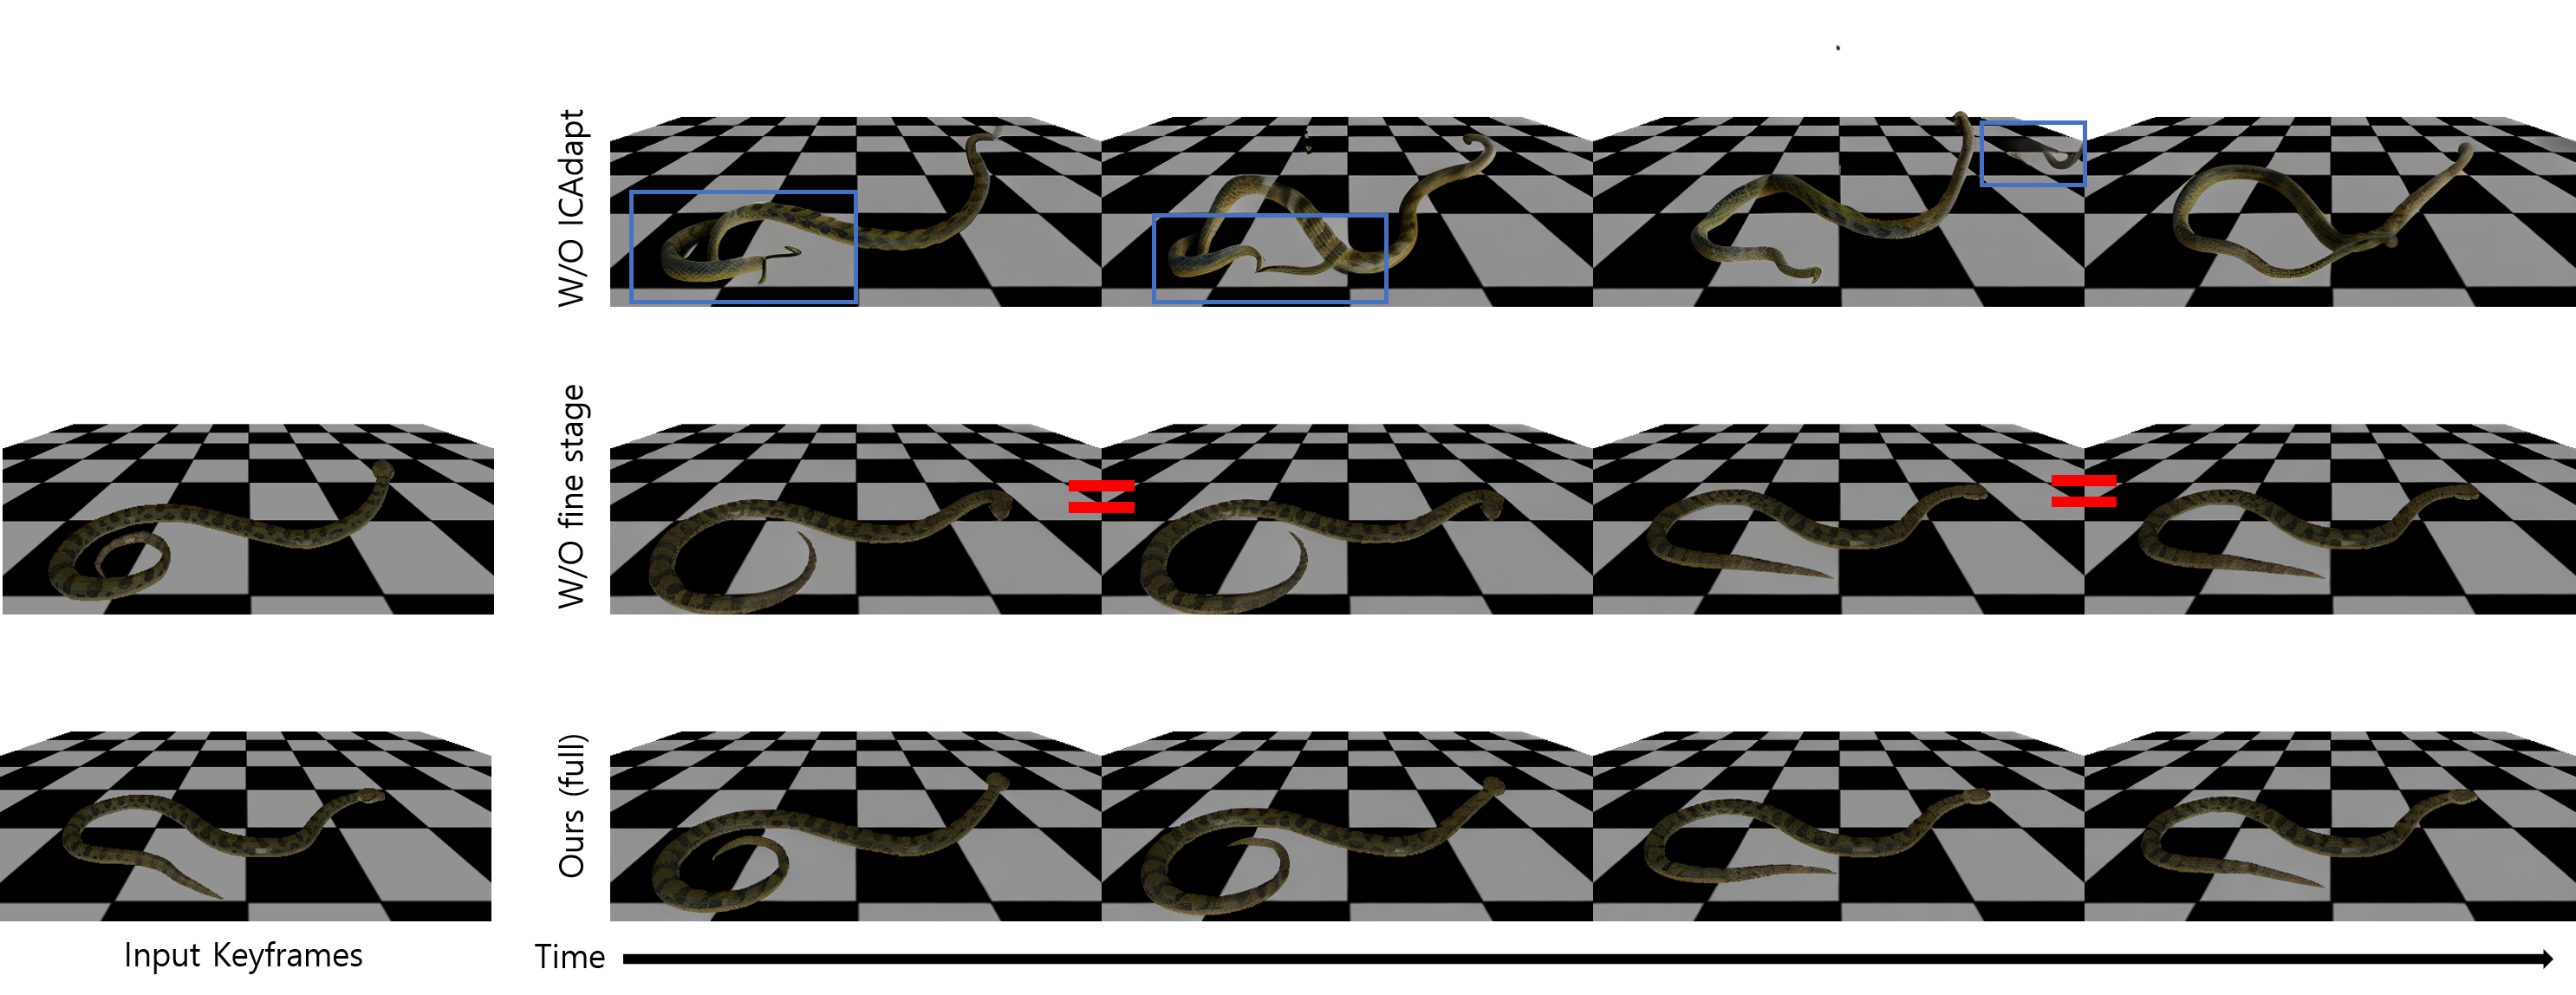}
\vspace{-6mm}
\caption{Additional results of the ablation study on video generation.}
\label{fig:x_video1}
\end{figure*}
\begin{figure*}[t]
\centering
\includegraphics[width=\linewidth]{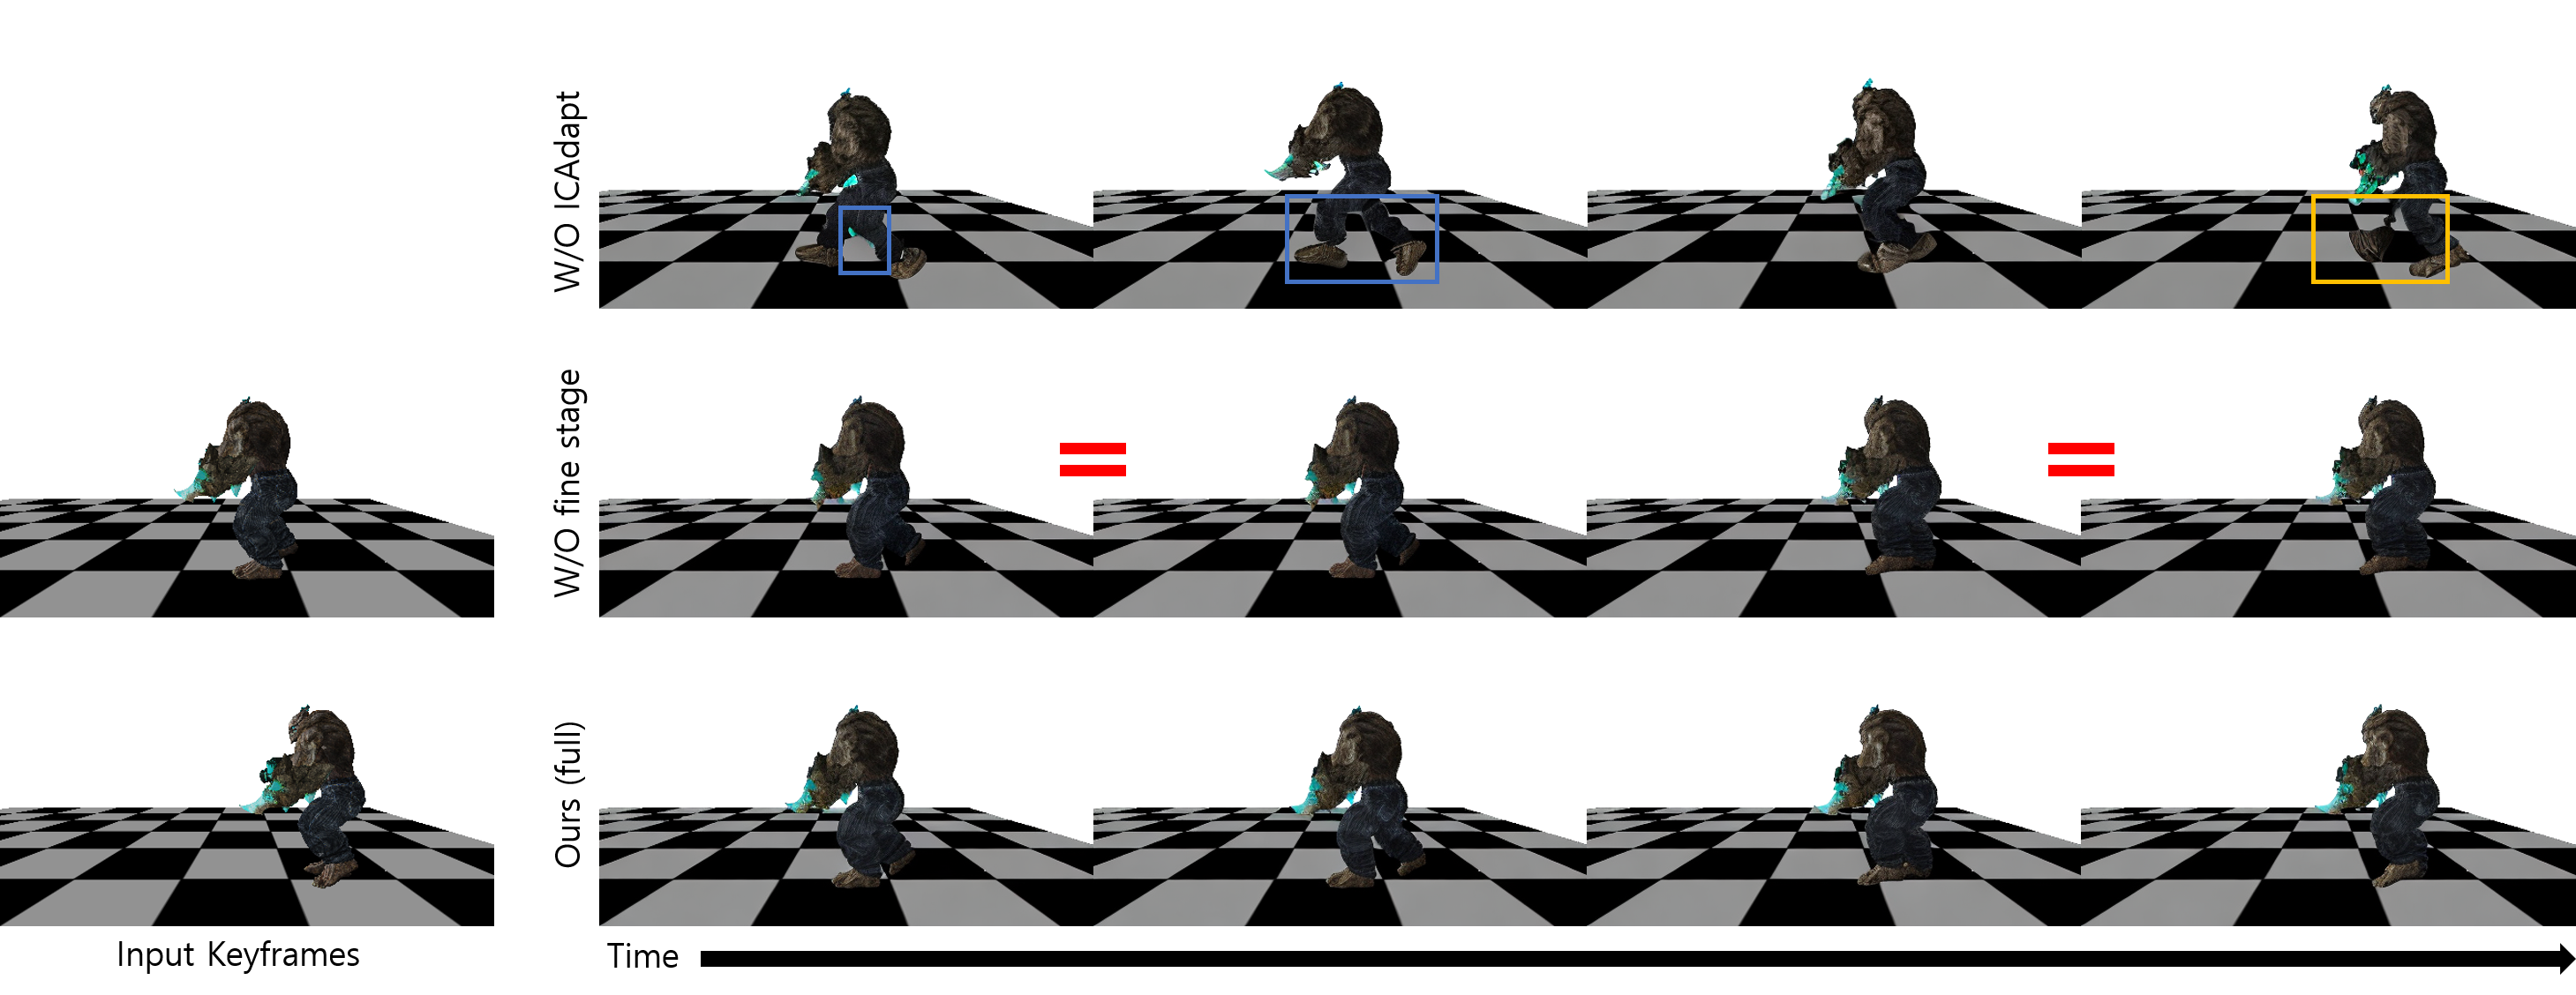}
\vspace{-6mm}
\caption{Additional results of the ablation study on video generation.}
\label{fig:x_video2}
\end{figure*}

Our scene-specific joint estimator, $\mathcal{E}_{scene}$, consists of a feature merger, heatmap decoder, and depth MLP. As shown in Figure~\ref{fig:x_joint}, our feature merger consists of convolutional blocks and concatenation. The output of the feature merger, $F$, serves as input for both 2D joints and per-joint depth estimation. The heatmap decoder consists of convolutional blocks with residual layers~\cite{he2016deep}. Here, we use a zero-initialized convolutional block for the residual connection.

The heatmap decoder outputs heatmaps with the channel size equal to the number of joints, $H \in \mathbb{R}^{B \times N_j \times w_h \times h_h}$, where $B$ is the size of the batch, $N_j$ is the number of channels, which corresponds to the number of joints, and $w_h$ and $h_h$ correspond to width and height, respectively. The heatmap becomes the position of the estimated 2D joint positions, $J_{2D} \in \mathbb{R}^{B \times N_j \times 2}$. We concatenate joint index embedding, $e_{joint} \in \mathbb{R}^{B \times N_j \times 1}$, which is analogous to positional embedding, to the 2D joint to provide an additional cue for estimating the depth of each joint. Afterwards, as described in the main paper, we sample the feature $f_{x,y} \in \mathbb{R}^{B \times 1 \times 1 \times C}$ for each joint from $F \in \mathbb{R}^{B \times w_F \times h_F \times C}$. Here, $w_F$ and $h_F$ are the width and height of feature $F$, and $C$ is the number of channels. Because $f_{x,y}$ is sampled for each joint, we concatenate and reshape these per-joint features to be $f_{processed} \in \mathbb{R}^{BN_j \times C}$. We reshape the 2D joint position and its joint index embedding to be per-joint values, $J_{processed2D} \in \mathbb{R}^{BN_j \times 3}$. We concatenate all of these sampled features, 2D joint positions, and index embeddings and pass them through the Depth MLP to estimate the per-joint depth values.

\begin{figure*}[t]
\centering
\includegraphics[width=0.95\linewidth]{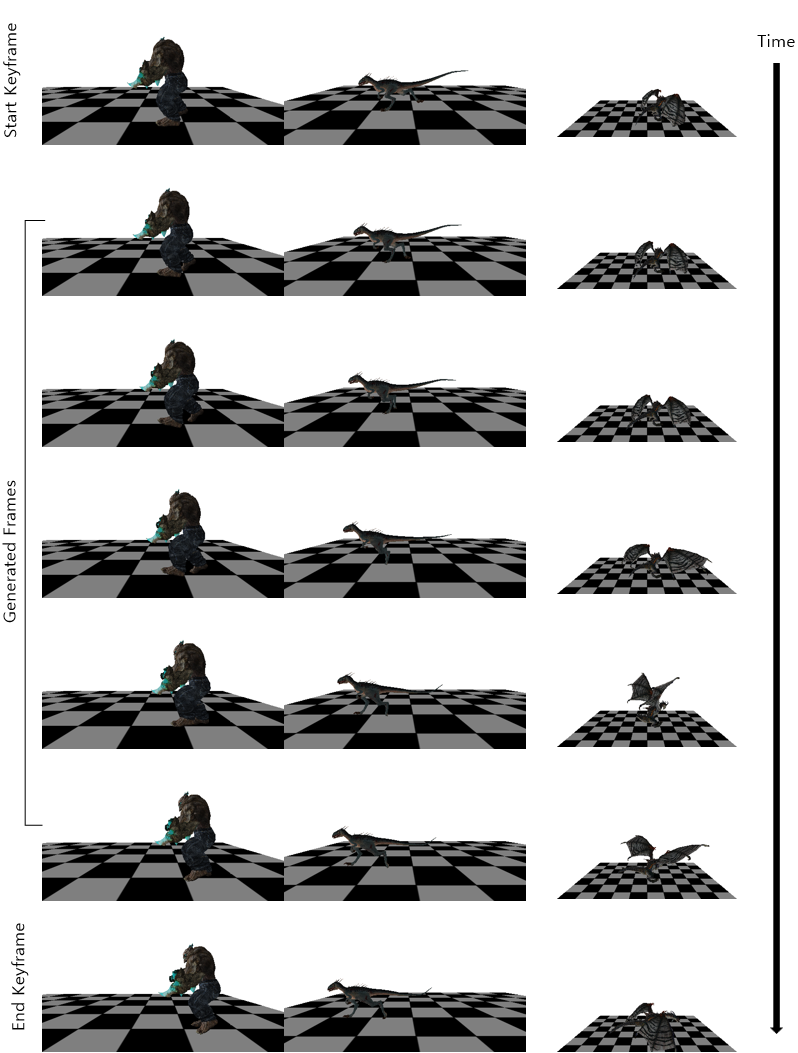}
\caption{Visual results of generated in-between motion frames.}
\label{fig:x_gen1}
\end{figure*}
\begin{figure*}[t]
\centering
\includegraphics[width=0.95\linewidth]{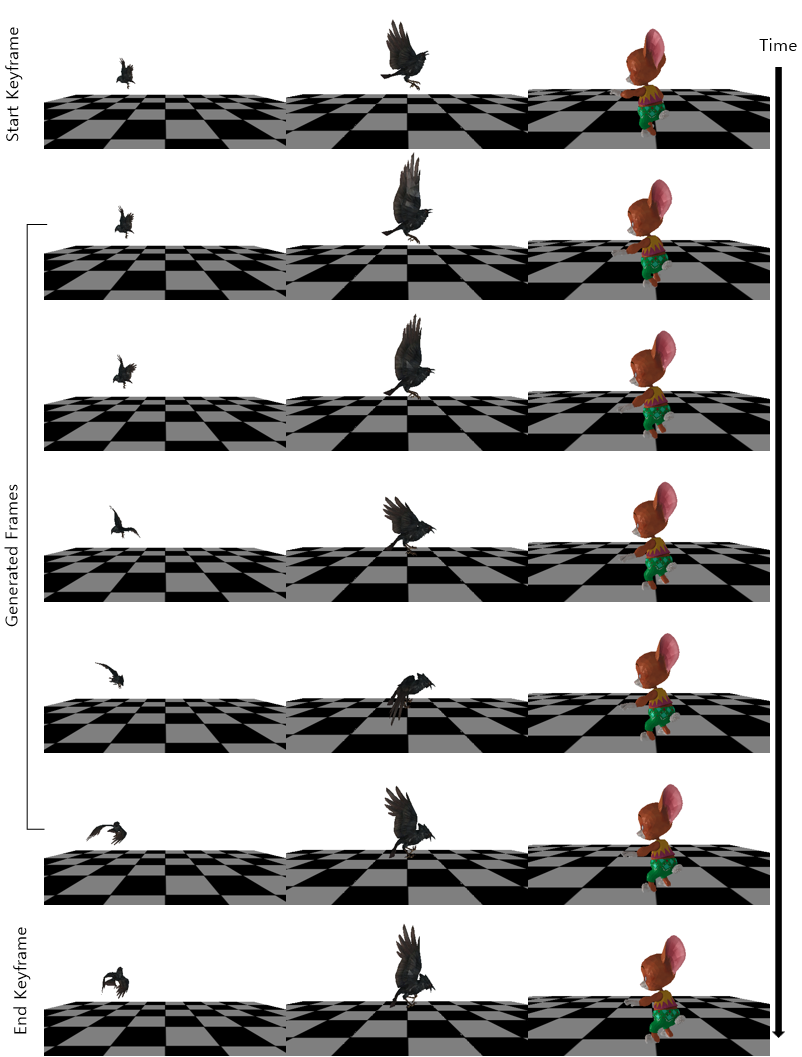}
\caption{Visual results of generated in-between motion frames.}
\label{fig:x_gen2}
\end{figure*}
\section*{C. Additional Results}\label{sec:C}

\begin{table*}
\centering
 % increase row height
\setlength{\tabcolsep}{4pt}
\caption{Quantitative results of H2Q variants and L2Q. Best scores are denoted in bold.}\vspace{-1mm}
\begin{tabular}{|l|cccc|cccc|}\hline
Character & \multicolumn{4}{c|}{Humanoid} & \multicolumn{4}{c|}{Non-humanoid}\\ 
\hline
Methods & HL2Q (1/4)$\downarrow$ & HL2Q$\downarrow$ & HL2Q (3/4)$\downarrow$ & L2Q$\downarrow$ & HL2Q(1/4)$\downarrow$ & HL2Q$\downarrow$ & HL2Q (3/4)$\downarrow$ & L2Q$\downarrow$ \\ \hline
Ours & \textbf{0.0019} & \textbf{0.0015} & \textbf{0.0014} & \textbf{0.0011} & \textbf{0.0016} & \textbf{0.0019} & \textbf{0.0024} & \textbf{0.0021} \\
SinMDM & 0.1526 & 0.0971 & 0.0636 & 0.0386 & 0.3664 & 0.2465 & 0.1979 & 0.1710 \\
SinMDM* & 0.1539 & 0.0981 & 0.0645 & 0.0390 & 0.3667 & 0.2467 & 0.1982 & 0.1713 \\
TST & 0.0028 & 0.0028 & 0.0069 & 0.0106 & - & - & - & - \\
ERQ-QV & 0.0031 & 0.0028 & 0.0064 & 0.0109 & - & - & - & - \\
\hline
\end{tabular}
\label{Tab:x_quant}
\end{table*}

We provide additional quantitative values computed by the HL2Q metric with varying thresholds: 1/4, 1/2, 3/4, and full in Table~\ref{Tab:x_quant}. The "full" threshold corresponds to the original L2Q, while the "1/2" threshold indicates what we used as HL2Q in the main paper. Our method produced the best results across all variants of HL2Q and L2Q. For humanoid characters, HL2Q values decreased as the filtering threshold became larger, indicating that the rotations were more precise at the near-leaf joints. However, no distinct pattern or difference was observed for non-humanoid characters.

For additional qualitative results, we first present the results of further visual ablation studies on video generation. As shown in Figures~\ref{fig:x_video1} and~\ref{fig:x_video2}, our method generated videos with smooth motion and no visible artifacts. Additionally, we visualized the results of Anymole on motion in-betweening in Figures~\ref{fig:x_gen1} and \ref{fig:x_gen2}.
